# Supplementary material for: Characterizing signal propagation to close the performance gap in unnormalized ResNets
Source: arXiv:2101.08692 source file (2021-01-27)
Supplement: Supplementary file 1 [file Appendix_FLOPs.tex]

How do we count flops? Previous work doesn't elaborate much on how these are counted, so we explain here.
